# Supplementary material for: Computing 3D chromatin configurations from contact probability maps by Inverse Brownian Dynamics
Source: arXiv:2002.09171 ancillary file (2020-02-21)
Supplement: Supplementary file 1 [file Supporting_Material.pdf]

# Supporting Material

## Computing 3D chromatin configurations from contact probability maps by Inverse Brownian Dynamics

K. Kumari, B. Dünweg, R. Padinhateeri, J. R. Prakash

## S1 Inverse Brownian dynamics

This section discusses the implementation of the Inverse Brownian Dynamics (IBD) method in the context of chromatin. The phase-space variable ($\Gamma$) for the coarse-grained bead-spring chain used to represent chromatin is the set of bead position vectors $\boldsymbol{r}_\mu(\mu = 1, 2, ..., N)$ and the Hamiltonian $\mathcal{H}(\Gamma, \{\epsilon_{\mu\nu}\}) = U^{\text{s}*} + U^{\text{SDK}*}$, where $U^{\text{s}*} = \sum_{\mu=1}^{N-1} U_\mu^{\text{s}*}$ and $U^{\text{SDK}*} = \sum_{\mu,\nu=1}^{N} U_{\mu\nu}^{\text{SDK}*}$. Since we are interested in bead-pairs, we construct a single index to represent any particular bead-pair. For instance, the expression

$$m = \frac{1}{2}[\mu(\mu - 1)] + [\nu - (\mu - 1)] \tag{1}$$

converts any bead pair $(\mu, \nu)$ to a single index $m$. Here $\mu$ varies from 2 to $N$, and $\nu$ varies from 1 to $(\mu - 1)$ for a matrix of size $N$. In terms of the single index, the average contact probability $p_m$ of the bead-pair $m$ is given by

$$p_m = \langle \hat{p}_m \rangle = \frac{1}{Z} \int d\Gamma \, \hat{p}_m \exp(-\beta \mathcal{H}) \tag{2}$$

Here, the partition function $Z = \int d\Gamma \exp(-\beta\mathcal{H})$, and $\hat{p}_m$ is an indicator function which indicates when contact occurs between the bead pair represented by index $m$. $\hat{p}_m$ is 1 if the distance between the beads is less than the cut-off distance of the indicator function, $r_{\text{p}}^*$, and 0 otherwise. For this work $r_{\text{p}}^* = r_{\text{c}}^*$, the cut-off distance of the SDK potential. We intend to target the experimentally obtained contact probability $p_m^{\text{ref}}$ by adjusting the well-depth of SDK attractive interactions $\epsilon_m$. The Taylor series expansion of $\langle \hat{p}_m \rangle$ about the interaction strength $\epsilon_m$ after neglecting higher order terms is

$$\langle \hat{p}_m \rangle(\epsilon_m + \Delta\epsilon_m) = \langle \hat{p}_m \rangle \, (\epsilon_m) + \sum_n \chi_{mn} \, \Delta\epsilon_n \tag{3}$$

where $\Delta\epsilon_m$ is the change in the interaction strength, and the susceptibility matrix

$$\chi_{mn} = \frac{\partial \langle \hat{p}_m \rangle}{\partial \epsilon_n} = \frac{\partial}{\partial \epsilon_n} \left[ \frac{1}{Z} \int d\Gamma \hat{p}_m \exp(-\beta\mathcal{H}) \right] \tag{4}$$

Simplifying further

$$\chi_{mn} = \frac{1}{Z}\left[\int \hat{p}_m \frac{\partial}{\partial \epsilon_n}\left(\exp(-\beta\mathcal{H})d\Gamma\right)\right] - \left[\frac{1}{Z}\left(\frac{1}{Z}\int \hat{p}_m \exp(-\beta\mathcal{H})d\Gamma\right)\frac{\partial Z}{\partial \epsilon_m}\right] \tag{5}$$

or

$$\chi_{mn} = \frac{\beta}{Z}\left[\int \hat{p}_m \exp(-\beta\mathcal{H})\frac{\partial(-\mathcal{H})}{\partial \epsilon_n}d\Gamma\right] - \beta\left[\langle \hat{p}_m\rangle \frac{1}{Z}\int \exp(-\beta\mathcal{H})\frac{\partial(-\mathcal{H})}{\partial \epsilon_n}d\Gamma\right], \tag{6}$$

Defining the quantity $b_n$ by

$$b_n = -\frac{\partial \mathcal{H}}{\partial \epsilon_n} \tag{7}$$

and using the expression for SDK potential, since only $U_n^{\mathrm{SDK}*}$ depends on $\epsilon_n$, one can show

$$b_n = \begin{cases} 1 & r_n^* \leq 2^{\frac{1}{6}}\sigma^* \\ \frac{1}{2}\left[1-\cos(\alpha\, r_n^{*2}+\beta)\right] & 2^{\frac{1}{6}}\sigma^* \leq r_n^* \leq r_{\mathrm{c}}^* \\ 0 & r_n^* \geq r_{\mathrm{c}}^* \end{cases} \tag{8}$$

which leads to

$$\chi_{mn} = \beta\left[\frac{1}{Z}\int \hat{p}_m b_n \exp(-\beta\mathcal{H})d\Gamma - \langle \hat{p}_m\rangle\frac{1}{Z}\int b_n \exp(-\beta\mathcal{H})d\Gamma\right] = \beta\left[\langle \hat{p}_m b_n\rangle - \langle \hat{p}_m\rangle\langle b_n\rangle\right] \tag{9}$$

Replacing the left hand side of Eq. 3 with the target contact probability $p_m^{\mathrm{ref}}$ obtained from experiment, we get

$$p_m^{\mathrm{ref}} - \langle \hat{p}_m\rangle = \sum_n \chi_{mn}\,\Delta\epsilon_n \tag{10}$$

Equation 10 can be solved for any particular iteration step as

$$\epsilon_n^{(i+1)} = \epsilon_n^{(i)} + \lambda\sum_m C_{nm}^{(i)}\left(p^{\mathrm{ref}} - \langle \hat{p}_m\rangle^{(i)}\right) \tag{11}$$

where the matrix $\mathsf{C}$ is the *pseudo-inverse* of the matrix $\chi$, superscript $i$ represents the iteration number, $\lambda$ denotes the damping factor with $0 < \lambda < 1$, and $\epsilon_n^{(i+1)}$ is the well-depth of the SDK attractive interaction for the next iteration step. Since the susceptibility matrix $\chi$ is often singular (with the rank of the matrix being smaller than its size), it is necessary to define the matrix $\mathsf{C}$ as a *pseudo-inverse* and determine it by using *singular-value decomposition* (SVD). By carrying out SVD, the susceptibility matrix is decomposed into three square matrices $\mathsf{U}, \mathsf{S}$ and $\mathsf{V}$ such that $\chi = \mathsf{U}\mathsf{S}\mathsf{V}^{\mathrm{T}}$ where $\mathsf{U}$ and $\mathsf{V}$ are orthogonal and $\mathsf{S}$ is a

diagonal matrix. The *pseudo-inverse* of the susceptibility matrix via SVD can then be written as

$$\mathsf{C} = \chi^{-1} = \mathsf{V} \cdot [\mathrm{diag}(1/S_n)] \cdot \mathsf{U}^T \tag{12}$$

Note that in all the cases considered here, $\chi, \mathsf{S}, \mathsf{U}$ and $\mathsf{V}$ are square matrices since there is a one-to-one correspondence between contact probability and interaction strength. As per the well-established procedure for finding the *pseudo-inverse*, when $S_n < 10^{-4}$, $1/S_n$ is replaced by 0. In other words, some values in the $\mathsf{S}$ matrix whose inverse would lead to problems, are ignored.

An example of the $\mathsf{S}$ matrix obtained in the case of the prototype scenario where we have considered a bead-spring chain with 45 beads is given here as illustration. The matrix is of size $N(N-1)/2 \times N(N-1)/2 = 990 \times 990$, which represent the number of interacting bead-pairs in the chain. Fig. S1 represents the matrix at an intermediate stage in the iteration process. It can been seen that $\mathsf{S}$ has diagonal elements whose magnitude is of order $10^{-4}$ or less (top right in Fig S1).

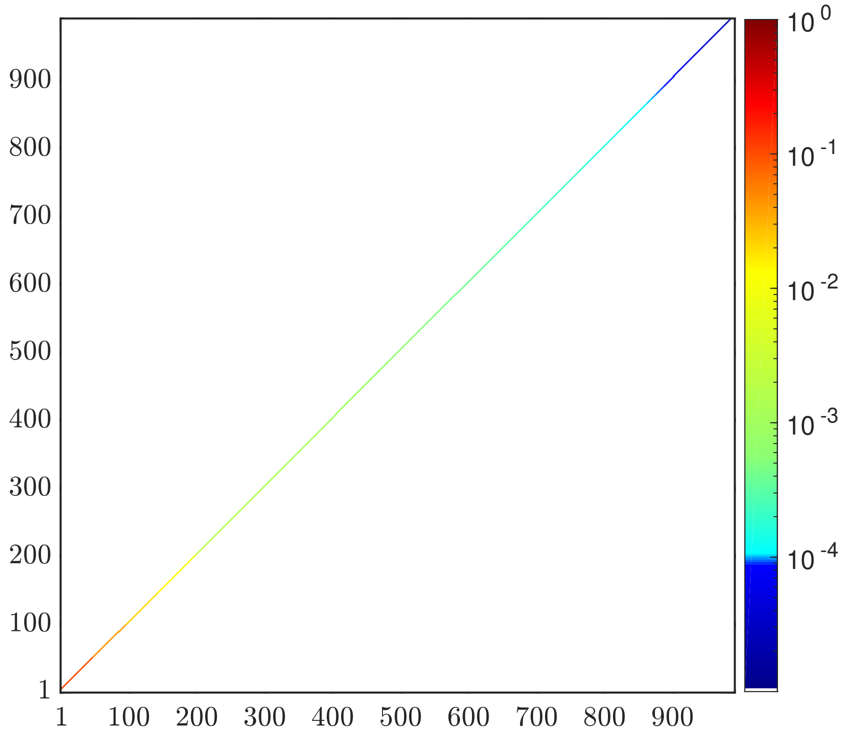


**Figure S1:** Representation of the matrix $\mathsf{S}$. The top right corner along the diagonal represents diagonal elements of the matrix, $S_n$, which are of order $10^{-4}$ or less.

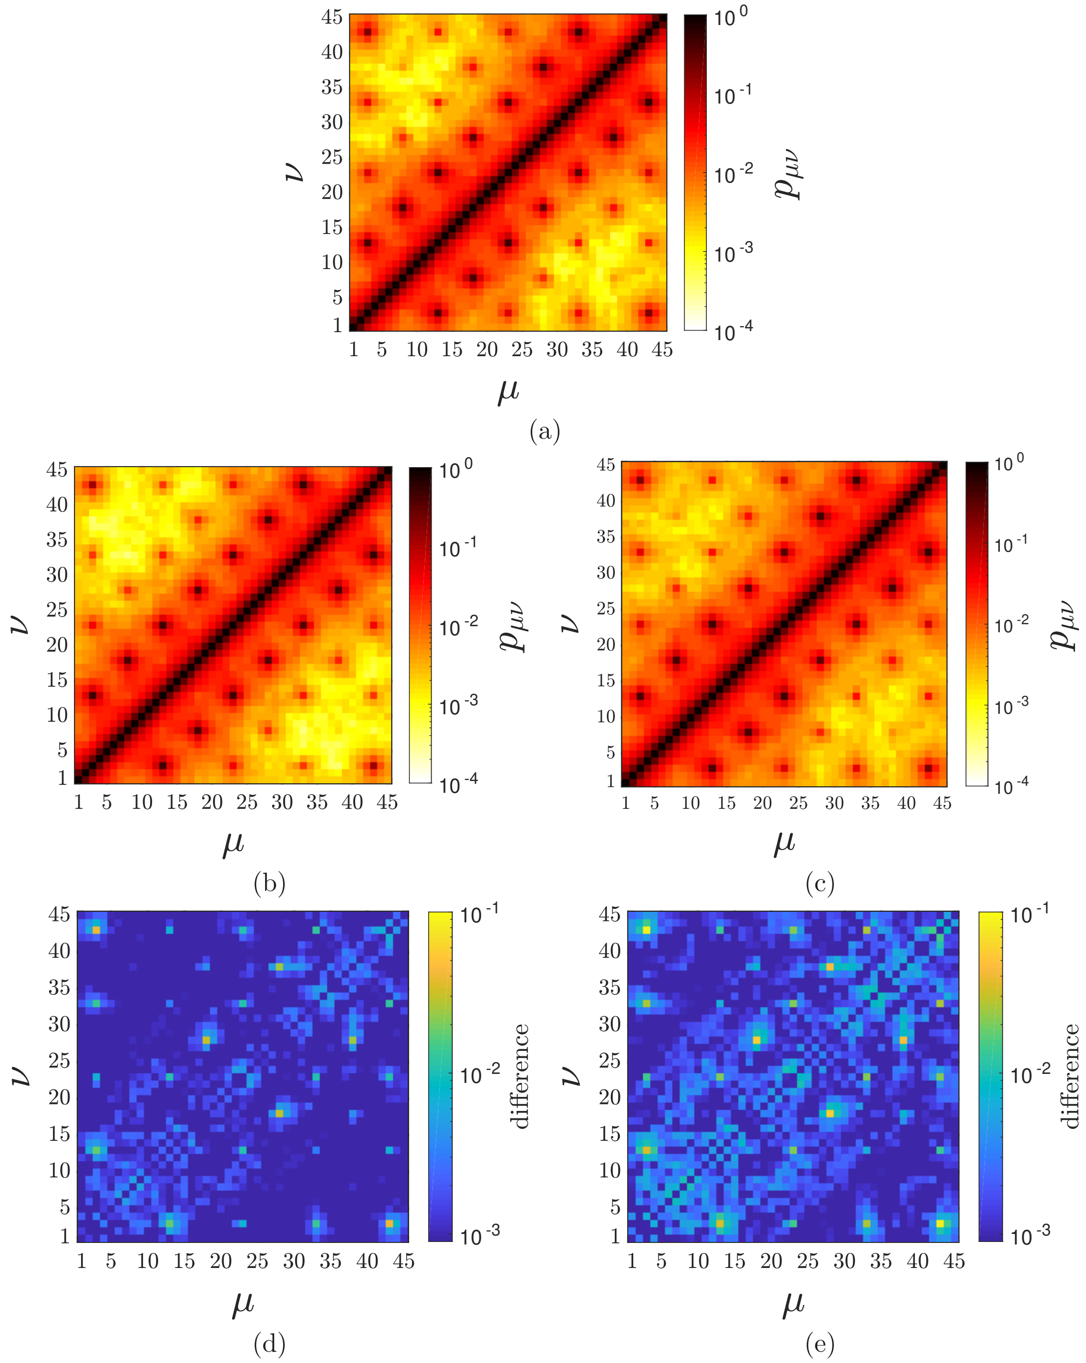


**Figure S2:** Validation of the IBD method with a prototype bead-spring chain with 45 beads. (a) Reference contact probability matrix. Two different initial states have been considered for testing IBD convergence, i.e., self-avoiding walk (SAW) where no bead-pairs have attractive interaction and the collapsed state where all the bead-pairs have attractive interaction, $\epsilon = 1$. (b) and (c) show the recovered contact probability matrix through IBD starting with SAW and collapsed state, respectively. The difference between the reference and recovered contact probability for each bead-pairs are shown for simulations starting from (d) self-avoiding walk and (e) collapsed state.

# S2 IBD validation for the prototype model

The robustness of the IBD algorithm, in the context of the prototype model, has been investigated in the main text by comparing the recovered contact probability matrix with the reference contact

probability matrix, starting from two different initial states, i.e., (i) a self-avoiding walk and (ii) a collapsed globule, as displayed in Figs. 2(b), 2(d) and 2(f). These figures are reproduced here for ease of reference, with Fig. S2(a) showing the reference contact probability matrix, while Figs. S2(b) and S2(c) show the recovered contact probability matrices starting from the self-avoiding walk and the collapsed polymer, respectively. Note that each of these recovered states has a root mean-squared deviation $E_{\rm rmsd}$ less than the pre-determined tolerance value. In addition to this data, here we show the *difference* in the reference and recovered contact probabilities, in the form of heatmaps which describe all bead pairs, for a self-avoiding walk in Fig. S2(d) and for the collapsed globule in Fig. S2(e). It is evident that higher differences are associated with higher contact probabilities, while the lower contact probabilities have minimal differences between the reference and recovered states.

It is interesting to examine how the polymer chain converges from different initial configurations (swollen or collapsed) to the final reference state of the prototype model. Note that the reference contact probabilities for the prototype model were produced with the interaction strength $\epsilon_{\mu\nu} = 7$ for eight bead-pairs, and with $\epsilon_{\mu\nu} = 0$ for all the remaining 982 bead-pairs. On the other hand, we set $\epsilon_{\mu\nu} = 0$ for all bead-pairs in the swollen state, and $\epsilon_{\mu\nu} = 1$ for all bead-pairs in the collapsed state. The value of 7 chosen for the interaction parameter $\epsilon_{\mu\nu}$ of the 8 bead-pairs in the prototype model has no particular significance. It has been chosen arbitrarily such that a high contact probability is obtained between some bead-pairs, as displayed in Fig. S2(a). Snapshots of the initial swollen and collapsed states are shown in Figs. S3(a) and S3(b), while a snapshot of the final converged state corresponding to the reference state is shown in Fig. S3(c). It is clear that while some beads in the reference state appear tightly bound, most of the others repel each other. Figure S3(d) displays the radius of gyration as a function of number of iterations in the IBD algorithm, as the system goes from the initial (swollen or collapsed) state to the final (reference) state. Starting from an initial swollen state, the radius of gyration decreases monotonically to the final state, defined by the contact probabilities in Fig. S2(a). When the starting state is the collapsed polymer, the radius of gyration increases monotonically until it reaches the final state. As is clear from the snapshot of the reference state, since the majority of the bead-pairs have no attraction, the reference state has a higher radius of gyration than the collapsed state. It is possible that some “strand passage” occurs in the neighbourhood of the tightly bound beads in the reference state as the chain conformation evolves from the initial collapsed state (where all the beads are attracted to each other) to the final reference state with a few tightly bound beads, since the current algorithm permits such passage (as discussed in section 2.1). The overall conformational evolution, however, as demonstrated by the radius of gyration in Fig. S3(d), is likely to be dominated by expanding chain conformations since the majority of the beads repel each other.

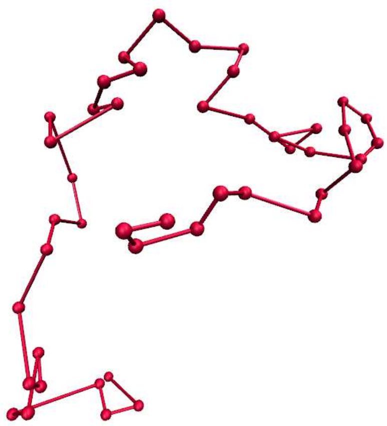

(a) initial state: swollen

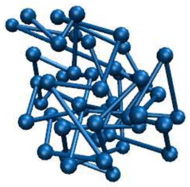

(b) initial state: collapsed

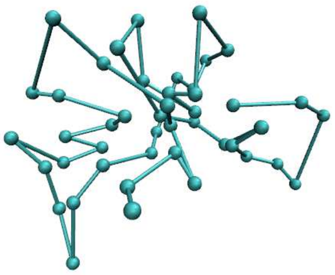

(c) reference state

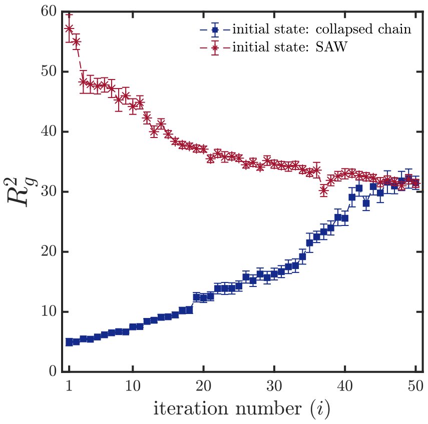


(d) radius of gyration

**Figure S3:** Randomly selected snapshots of (a) the swollen (self-avoiding walk) initial state (b) the collapsed initial state, and (c) the converged reference state. (d) Change in $R_g^2$ with the number of iterations in the IBD algorithm, as the system goes from initial (swollen or collapsed) state to the final (reference) state.

# S3 ICE normalization

ICED package (http://projects.cbio.mines-paristech.fr/iced) was used to normalize the contact count matrix of $\alpha$-globin gene locus (both K562 and GM12878 cell line). The whole matrix was then divided by the summation of the row (summation of each row is a constant after the ICE normalization) so that the contact probability for each bin sums to 1. Fig. S4(a) and S4(b) shows the ICE normalized matrix for

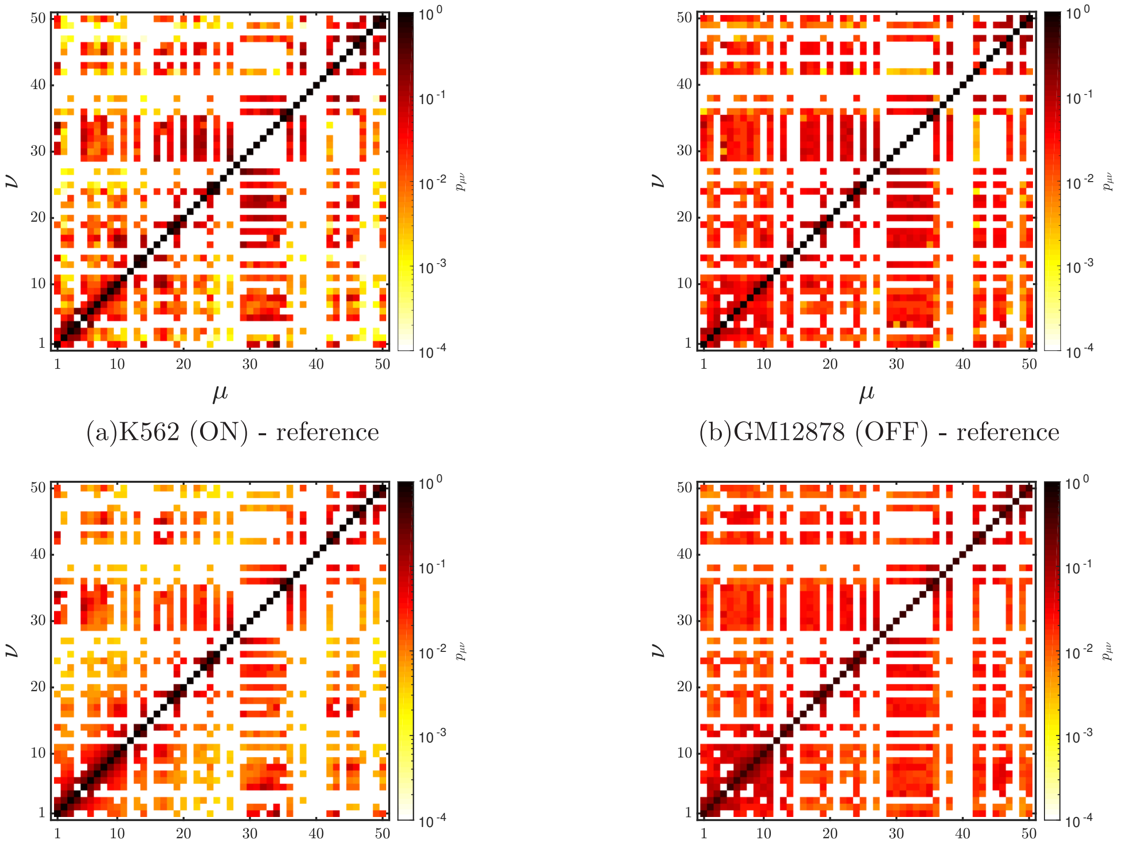


(a)K562 (ON) - reference (b)GM12878 (OFF) - reference

(c)K562 (ON) - recovered (d)GM12878 (OFF) - recovered

**Figure S4:** Comparison of the reference ICE normalized contact probabilities ((a) and (b)) with the recovered contact probabilities ((c) and (d)), obtained with the IBD method for K562 and GM12878, respectively.

K562 (ON state) and GM12878 (OFF state), respectively. To study the 3D configurations, we performed IBD on the ICE normalized contact counts matrix. The contact probabilities recovered in this process are represented in Fig. S4(c) and S4(d) for K562 and GM12878 cell line. It is evident from these figures that IBD algorithm has successfully recovered the ICE normalized contact matrix for both the states.

The spatial distances calculated for the contact probabilities in the ON and OFF state are shown in Fig. S5(a) for K562 (ON state) and in Fig. S5(b) for GM12878 (OFF state) cell lines. Each point in these figures represents the ensemble-averaged 3D distance between a given pair of beads ($y$-axis) having a contact probability as indicated in the $x$-axis. Similar to the $N_f = 0$ case, a wide range of 3D distances is possible and is also dependent on the distance along the contour between the beads ($|\mu - \nu|$). The red line in both the figures are fitted power-laws to the data and the dashed line (green and magenta) are chosen arbitrarily as a guide to the eye indicating the boundaries of spatial distance spread. The same data has been binned and plotted as violin plots that display the mean 3D distance for a given small range of contact probabilities, as shown in Figs. S6 (a) and (b). This distribution is observed to be very

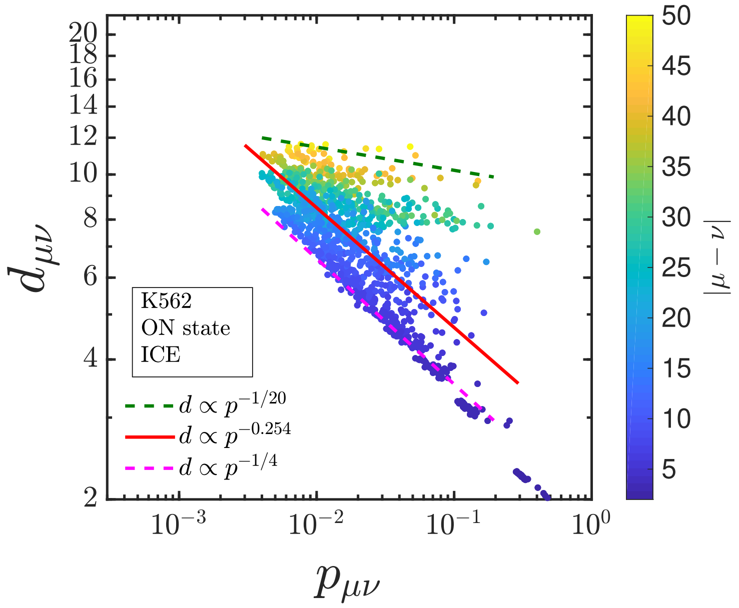


(a)

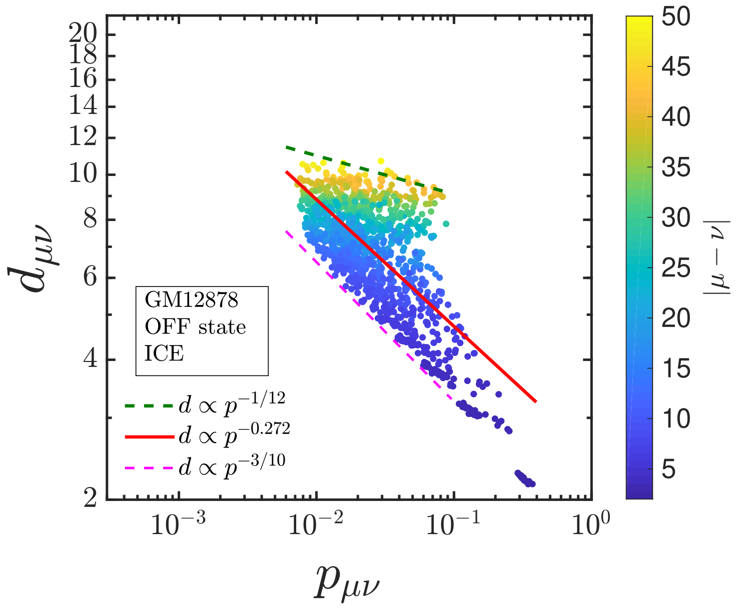


(b)

**Figure S5:** Dependence of mean 3D distances $d_{\mu\nu}$ on contact probabilities $p_{\mu\nu}$ for (a) K562 (ON state) and (b) GM12878 (OFF state) cell lines, respectively for ICE normalization. For the K562 (ON state) cell line, the contact probabilities are bounded by power laws, $d_{\mu\nu} \propto p^{\tau}_{\mu\nu}$, where $\tau$ varies from $-1/20$ (upper bound) to $-1/4$ (lower bound) as indicated by the green and magenta dashed line. Similarly, in the GM12878 (OFF state), $\tau$ varies from $-1/12$ to $-3/10$. The red line indicates the power law fitted to the simulation data points.

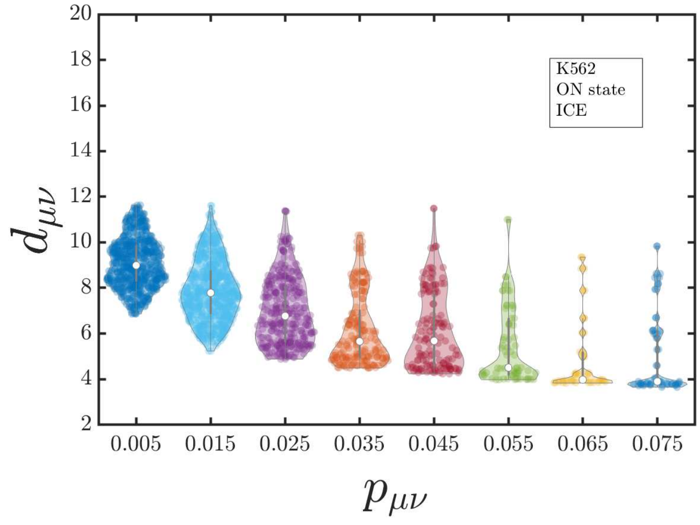


(a)

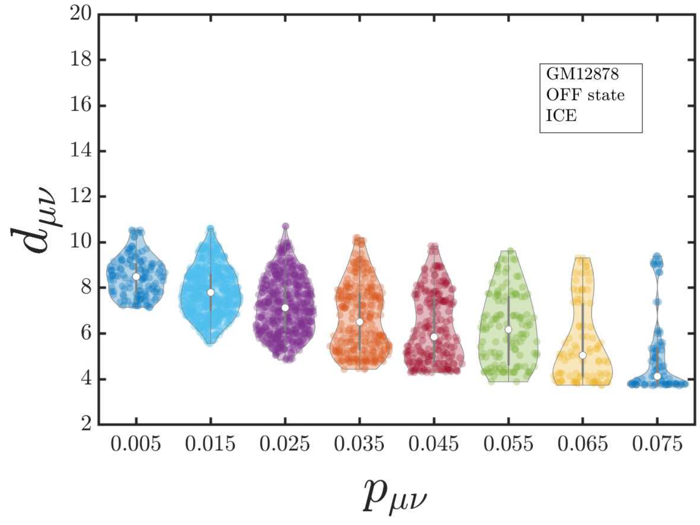


(b)

**Figure S6:** Violin plots which display the probability distribution of mean 3D distances for selected ranges of contact probabilities in (a) the K562 (ON state) cell lines, and (b) the GM12878 (OFF state) cell lines normalized with ICE.

different from the other simple normalization studied in the present work.

## S4 Additional data on density profile and contact probability

Data not provided in the main manuscript are given here in the supporting material for the sake of completeness.

As discussed earlier, three coarse-grained techniques namely (i) *average*, (ii) *dependent* and (iii) *independent* have been used. It was seen previously that there was no influence of these coarse-graining techniques on the radius of gyration ($R_g$). Similarly, it is clear from Fig. S7, that there is no influence

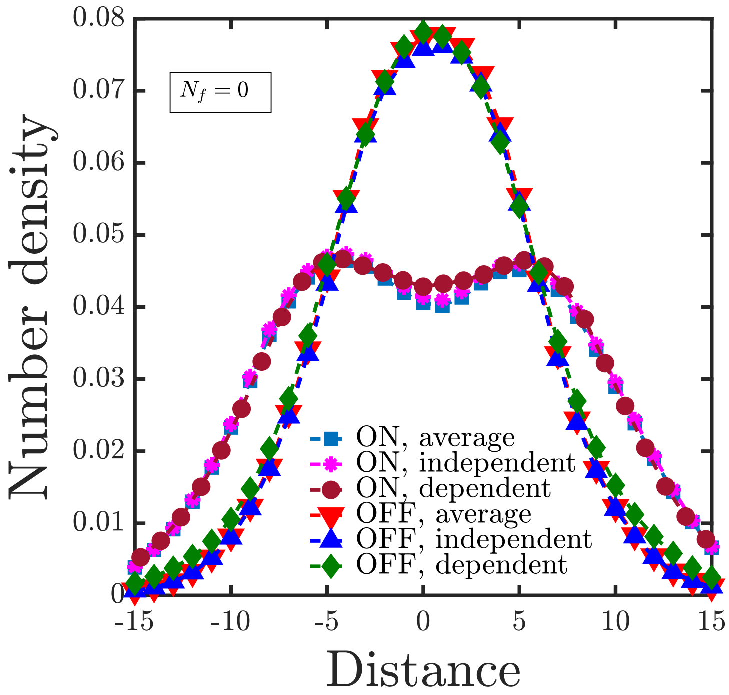


**Figure S7:** Comparison of the number density of beads along the major axis of the radius of gyration tensor, for both the cell line K562 and GM12878 with three coarse-graining techniques i.e *dependent*, *independent* and *average*.

of coarse-graining technique on density profile either.

The spatial distances relationship with contact probabilities at $N_f = 1$ are shown in Fig. S8(a) for K562 (ON state) and in Fig. S8(b) for GM12878 (OFF state) cell lines. Each point in these figures represents the ensemble-averaged 3D distance between a given pair of beads ($y$-axis) having a contact probability as indicated in the $x$-axis. The color variation in Figs. S8(a) and (b) indicates the influence of contour length. The red line in both the figures is fitted power-laws to the data. The dashed line (green and magenta) are chosen arbitrarily as a guide to the eye, indicating the boundaries of spatial distance spread. The same data has been binned and plotted as violin plots that display the mean 3D distance for a given small range of contact probabilities, as shown in Figs. S9 (a) and (b). As the distribution of points around the mean is very diverse again supports that a simple functional form between the mean 3D distance and the contact probability may not be feasible.

The value of interaction strength parameter $\epsilon_{\mu\nu}$ for K562 (ON state) and GM12878 (OFF state) cell lines at the converged state were shown in Fig.3. However. the exact values of the optimized interaction strength $\epsilon_{\mu\nu}$ for all the bead pairs are provided in Table S1 for GM12878 and in Table S2 for K562 cell line.

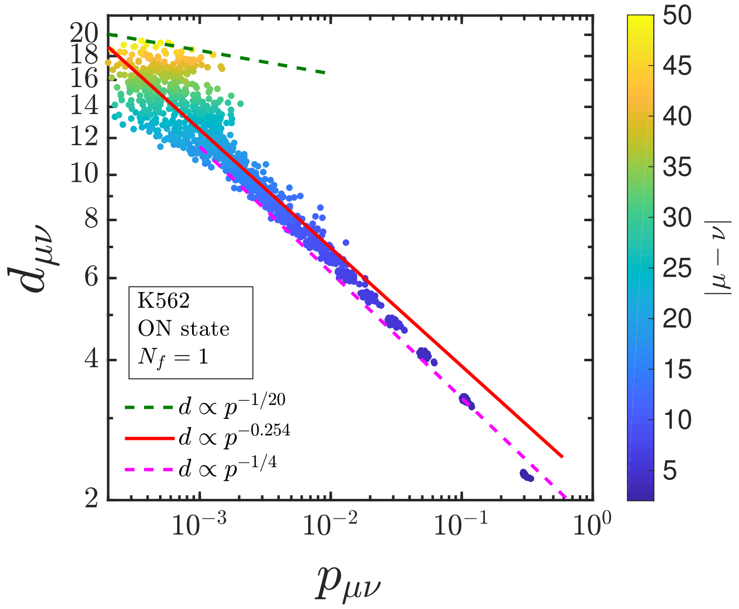


(a)

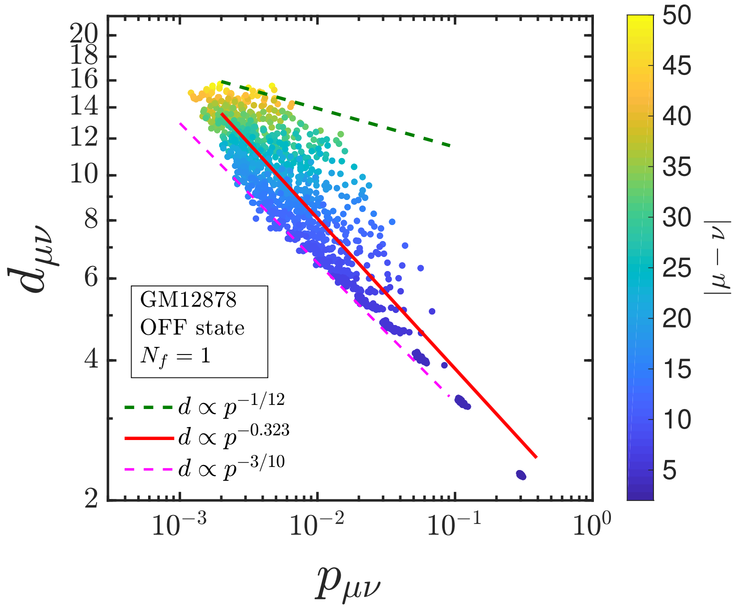


(b)

**Figure S8:** Dependence of mean 3D distances $d_{\mu\nu}$ on contact probabilities $p_{\mu\nu}$ for (a) K562 (ON state) and (b) GM12878 (OFF state) cell lines, respectively at $N_f = 1$. For the K562 (ON state) cell line, the contact probabilities are bounded by power laws, $d_{\mu\nu} \propto p^{\tau}_{\mu\nu}$, where $\tau$ varies from $-1/20$ (upper bound) to $-1/4$ (lower bound) as indicated by the green and magenta dashed line. Similarly, in the GM12878 (OFF state), $\tau$ varies from $-1/12$ to $-3/10$. The red line is fitted to the data points.

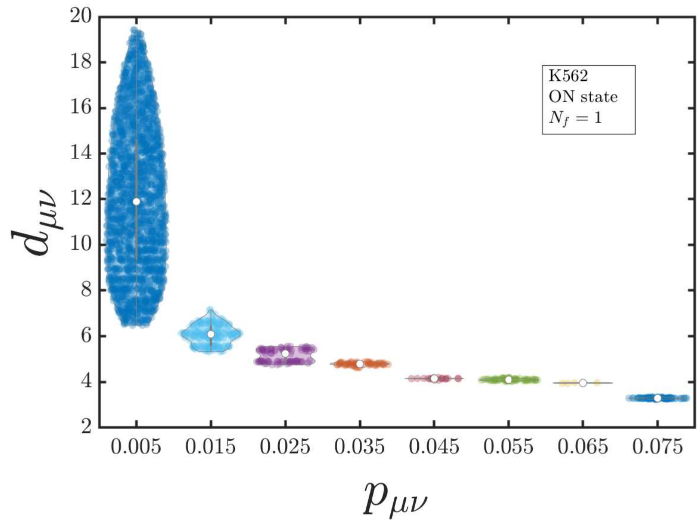


(a)

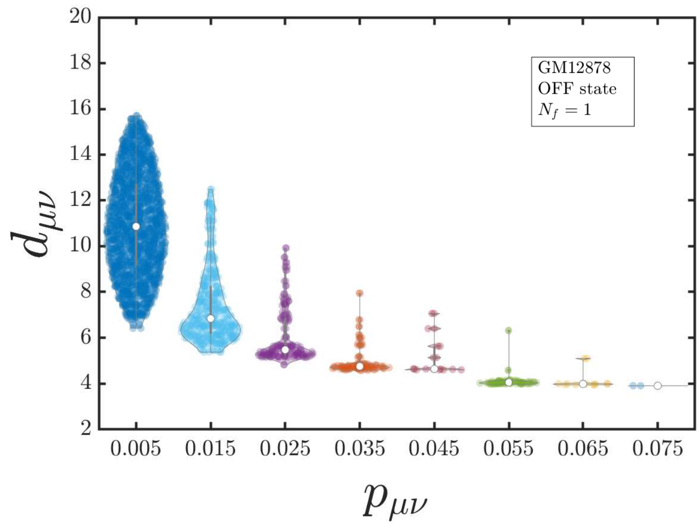


(b)

**Figure S9:** Violin plots showing the probability distribution of mean 3D distances for selected ranges of contact probabilities in (a) the K562 (ON state) cell lines, and (b) the GM12878 (OFF state) at normalization factor $N_f = 1$.

**Table S1:** Optimized interaction strength matrix for GM12878 (OFF state) cell line at the normalizing factor $N_f = 0$. The first row and the first column indicates the bead number ($\mu$ or $\nu$) and all the remaining elements represent the attractive strength between the corresponding bead pairs ($\epsilon_{\mu\nu}$).

| | 1 | 2 | 3 | 4 | 5 | 6 | 7 | 8 | 9 | 10 | 11 | 12 | 13 | 14 | 15 | 16 | 17 |
|---|---|---|---|---|---|---|---|---|---|---|---|---|---|---|---|---|---|
| 1 | 0 | 0 | 0 | 0 | 0 | 0 | 0 | 0 | 0 | 0.27 | 0 | 0 | 0 | 0 | 0 | 0 | 0 |
| 2 | 0 | 0 | 0 | 0 | 0.34 | 0.15 | 1.13 | 0.09 | 1.4 | 1.87 | 1.11 | 0 | 0.06 | 1.58 | 0 | 0 | 0 |
| 3 | 0 | 0 | 0 | 0 | 0.33 | 0.02 | 0.08 | 1.05 | 0.62 | 0 | 1.51 | 0 | 1.78 | 0 | 0 | 0.4 | 0 |
| 4 | 0 | 0 | 0 | 0 | 0 | 0 | 0 | 0 | 0 | 0 | 0 | 0 | 0 | 0 | 0 | 0 | 0 |
| 5 | 0 | 0.34 | 0.33 | 0 | 0 | 0 | 0 | 0 | 0.88 | 2.06 | 0.91 | 0 | 0 | 1.87 | 0 | 0 | 0 |
| 6 | 0 | 0.15 | 0.02 | 0 | 0 | 0 | 0 | 0 | 0 | 0.46 | 0.19 | 0 | 0 | 0.1 | 0 | 0 | 0 |
| 7 | 0 | 1.13 | 0.08 | 0 | 0 | 0 | 0 | 0 | 0 | 0.57 | 0 | 0 | 0.19 | 0.59 | 0 | 0 | 0 |
| 8 | 0 | 0.09 | 1.05 | 0 | 0 | 0 | 0 | 0 | 0 | 0 | 0 | 0 | 0 | 0.36 | 0 | 0 | 0 |
| 9 | 0 | 1.4 | 0.62 | 0 | 0.88 | 0 | 0 | 0 | 0 | 0.96 | 0 | 0 | 0.03 | 0.05 | 0 | 0 | 0 |
| 10 | 0.27 | 1.87 | 0 | 0 | 2.06 | 0.46 | 0.57 | 0 | 0.96 | 0 | 0.2 | 0 | 1.55 | 0 | 0 | 0.96 | 0.28 |
| 11 | 0 | 1.11 | 1.51 | 0 | 0.91 | 0.19 | 0 | 0 | 0 | 0.2 | 0 | 0 | 0 | 0.55 | 0 | 0 | 0 |
| 12 | 0 | 0 | 0 | 0 | 0 | 0 | 0 | 0 | 0 | 0 | 0 | 0 | 0 | 0 | 0 | 0 | 0 |
| 13 | 0 | 0.06 | 1.78 | 0 | 0 | 0 | 0.19 | 0 | 0.03 | 1.55 | 0 | 0 | 0 | 0.24 | 0 | 0 | 0 |
| 14 | 0 | 1.58 | 0 | 0 | 1.87 | 0.1 | 0.59 | 0.36 | 0.05 | 0 | 0.55 | 0 | 0.24 | 0 | 0 | 0 | 0 |
| 15 | 0 | 0 | 0 | 0 | 0 | 0 | 0 | 0 | 0 | 0 | 0 | 0 | 0 | 0 | 0 | 0 | 0 |
| 16 | 0 | 0 | 0.4 | 0 | 0 | 0 | 0 | 0 | 0 | 0.96 | 0 | 0 | 0 | 0 | 0 | 0 | 0 |
| 17 | 0 | 0 | 0 | 0 | 0 | 0 | 0 | 0 | 0 | 0.28 | 0 | 0 | 0 | 0 | 0 | 0 | 0 |
| 18 | 0 | 1.58 | 2.1 | 0 | 0 | 0.85 | 1.4 | 0 | 0.78 | 2.15 | 0.66 | 0 | 0 | 1.3 | 0 | 0 | 0 |
| 19 | 0 | 0.59 | 0 | 0 | 1.97 | 0 | 0 | 0.62 | 0 | 0 | 0.53 | 0 | 0.56 | 0 | 0 | 0 | 0 |
| 20 | 0 | 1.16 | 2.02 | 0 | 0 | 0.12 | 1.21 | 0 | 0.82 | 2.08 | 0.9 | 0 | 0 | 1.57 | 0 | 0 | 0 |
| 21 | 0 | 0 | 0 | 0 | 0 | 0 | 0 | 0 | 0 | 0 | 0 | 0 | 0 | 0 | 0 | 0 | 0 |
| 22 | 0 | 0.87 | 1.59 | 0 | 0 | 0 | 1 | 0 | 0.5 | 2.05 | 0.9 | 0 | 0 | 1.4 | 0 | 0 | 0 |
| 23 | 0 | 0 | 0 | 0 | 0 | 0 | 0 | 0 | 0 | 0 | 0 | 0 | 0 | 0 | 0 | 0 | 0 |
| 24 | 0.01 | 1.17 | 0 | 0 | 2.05 | 0.99 | 1.08 | 0.77 | 1.01 | 0 | 1.12 | 0 | 1.65 | 0 | 0 | 0.12 | 0 |
| 25 | 0 | 1.1 | 2.07 | 0 | 0 | 0 | 0.92 | 0 | 0.3 | 2.15 | 0.58 | 0 | 0 | 1.75 | 0 | 0 | 0 |
| 26 | 0 | 0 | 0 | 0 | 0 | 0 | 0 | 0 | 0 | 0 | 0 | 0 | 0 | 0 | 0 | 0 | 0 |
| 27 | 0 | 0 | 0.58 | 0 | 0 | 0 | 0 | 0 | 0 | 0.84 | 0 | 0 | 0 | 0 | 0 | 0 | 0 |
| 28 | 0 | 0 | 0 | 0 | 0 | 0 | 0 | 0 | 0 | 0 | 0 | 0 | 0 | 0 | 0 | 0 | 0 |
| 29 | 0 | 0.89 | 0 | 0 | 1.13 | 0.2 | 0.91 | 0.02 | 0.43 | 0 | 0.92 | 0 | 1.62 | 0 | 0 | 0.24 | 0 |
| 30 | 0 | 1.36 | 0 | 0 | 1.81 | 0.32 | 0.42 | 1.24 | 0.41 | 0 | 1.94 | 0 | 1.58 | 0 | 0 | 1.05 | 0 |
| 31 | 0.19 | 1.3 | 0 | 0 | 1.64 | 1.08 | 0.52 | 0.62 | 0.63 | 0 | 1.16 | 0 | 1.55 | 0 | 0 | 0.65 | 0 |
| 32 | 0.04 | 2.05 | 0 | 0 | 2 | 0 | 0.69 | 0.71 | 0.34 | 0 | 1.93 | 0 | 1.56 | 0 | 0 | 0.75 | 0 |
| 33 | 0 | 0 | 0 | 0 | 0.91 | 0 | 0 | 0 | 0.24 | 0 | 0.52 | 0 | 0 | 0 | 0 | 0 | 0 |
| 34 | 1.95 | 2 | 0 | 0 | 2.03 | 0.32 | 1.14 | 1.37 | 1.34 | 0 | 1.8 | 0 | 2.04 | 0 | 0 | 1.35 | 0.02 |
| 35 | 0 | 1.03 | 0 | 0 | 1.45 | 0 | 0.96 | 0 | 0 | 0 | 1.66 | 0 | 0.42 | 0 | 0 | 0 | 0 |
| 36 | 0 | 0.5 | 0.94 | 0 | 0 | 0 | 0.62 | 0 | 0.27 | 1.39 | 0.19 | 0 | 0 | 0.14 | 0 | 0.05 | 0 |
| 37 | 0 | 0 | 0 | 0 | 0 | 0 | 0 | 0 | 0 | 0 | 0 | 0 | 0 | 0 | 0 | 0 | 0 |
| 38 | 0 | 1.34 | 2.05 | 0 | 0 | 0 | 1.3 | 0 | 1.01 | 2.11 | 1.18 | 0 | 0 | 2.03 | 0 | 0 | 0 |
| 39 | 0 | 0 | 0 | 0 | 0 | 0 | 0 | 0 | 0 | 0 | 0 | 0 | 0 | 0 | 0 | 0 | 0 |
| 40 | 0 | 0 | 0 | 0 | 0 | 0 | 0 | 0 | 0 | 0 | 0 | 0 | 0 | 0 | 0 | 0 | 0 |
| 41 | 0 | 0 | 0 | 0 | 0 | 0 | 0 | 0 | 0 | 0 | 0 | 0 | 0 | 0 | 0 | 0 | 0 |
| 42 | 0.72 | 2.05 | 0 | 0 | 2.08 | 1.05 | 1.42 | 1.09 | 0.85 | 0 | 2.03 | 0 | 2.07 | 0 | 0 | 1.7 | 0 |
| 43 | 0.08 | 1.34 | 0 | 0 | 1.91 | 0 | 0 | 0.34 | 0.96 | 0 | 1.65 | 0 | 1.18 | 0 | 0 | 0.72 | 0 |
| 44 | 0 | 0 | 0 | 0 | 0 | 0 | 0 | 0 | 0 | 0 | 0 | 0 | 0 | 0 | 0 | 0 | 0 |
| 45 | 1.01 | 1.73 | 0 | 0 | 1.85 | 1.02 | 1.28 | 1.06 | 1.57 | 0 | 1.72 | 0 | 1.9 | 0 | 0 | 1 | 0 |
| 46 | 0 | 1.08 | 0 | 0 | 1.91 | 0 | 0 | 0.41 | 0.64 | 0 | 1.19 | 0 | 1.8 | 0 | 0 | 0.05 | 0 |
| 47 | 0 | 1.49 | 0.33 | 0 | 0 | 0 | 0.42 | 0 | 0.14 | 1.22 | 0 | 0 | 0 | 1.58 | 0 | 0 | 0 |
| 48 | 0 | 0 | 0 | 0 | 0 | 0 | 0 | 0 | 0 | 0 | 0 | 0 | 0 | 0 | 0 | 0 | 0 |
| 49 | 0 | 1.12 | 0.22 | 0 | 0 | 0 | 0 | 0 | 0 | 1.4 | 0.98 | 0 | 0 | 0.82 | 0 | 0.43 | 0 |
| 50 | 0.47 | 2.01 | 0 | 0 | 2.14 | 0.94 | 1.52 | 0.88 | 1.25 | 0 | 2.05 | 0 | 2.15 | 0 | 0 | 0.12 | 0 |

Continued table S1

| | 18 | 19 | 20 | 21 | 22 | 23 | 24 | 25 | 26 | 27 | 28 | 29 | 30 | 31 | 32 | 33 | 34 |
|---|---|---|---|---|---|---|---|---|---|---|---|---|---|---|---|---|---|
| 1 | 0 | 0 | 0 | 0 | 0 | 0 | 0.01 | 0 | 0 | 0 | 0 | 0 | 0 | 0.19 | 0.04 | 0 | 1.95 |
| 2 | 1.58 | 0.59 | 1.16 | 0 | 0.87 | 0 | 1.17 | 1.1 | 0 | 0 | 0 | 0.89 | 1.36 | 1.3 | 2.05 | 0 | 2 |
| 3 | 2.1 | 0 | 2.02 | 0 | 1.59 | 0 | 0 | 2.07 | 0 | 0.58 | 0 | 0 | 0 | 0 | 0 | 0 | 0 |
| 4 | 0 | 0 | 0 | 0 | 0 | 0 | 0 | 0 | 0 | 0 | 0 | 0 | 0 | 0 | 0 | 0 | 0 |
| 5 | 0 | 1.97 | 0 | 0 | 0 | 0 | 2.05 | 0 | 0 | 0 | 0 | 1.13 | 1.81 | 1.64 | 2 | 0.91 | 2.03 |
| 6 | 0.85 | 0 | 0.12 | 0 | 0 | 0 | 0.99 | 0 | 0 | 0 | 0 | 0.2 | 0.32 | 1.08 | 0 | 0 | 0.32 |
| 7 | 1.4 | 0 | 1.21 | 0 | 1 | 0 | 1.08 | 0.92 | 0 | 0 | 0 | 0.91 | 0.42 | 0.52 | 0.69 | 0 | 1.14 |
| 8 | 0 | 0.62 | 0 | 0 | 0 | 0 | 0.77 | 0 | 0 | 0 | 0 | 0.02 | 1.24 | 0.62 | 0.71 | 0 | 1.37 |
| 9 | 0.78 | 0 | 0.82 | 0 | 0.5 | 0 | 1.01 | 0.3 | 0 | 0 | 0 | 0.43 | 0.41 | 0.63 | 0.34 | 0.24 | 1.34 |
| 10 | 2.15 | 0 | 2.08 | 0 | 2.05 | 0 | 0 | 2.15 | 0 | 0.84 | 0 | 0 | 0 | 0 | 0 | 0 | 0 |
| 11 | 0.66 | 0.53 | 0.9 | 0 | 0.9 | 0 | 1.12 | 0.58 | 0 | 0 | 0 | 0.92 | 1.94 | 1.16 | 1.93 | 0.52 | 1.8 |
| 12 | 0 | 0 | 0 | 0 | 0 | 0 | 0 | 0 | 0 | 0 | 0 | 0 | 0 | 0 | 0 | 0 | 0 |
| 13 | 0 | 0.56 | 0 | 0 | 0 | 0 | 1.65 | 0 | 0 | 0 | 0 | 1.62 | 1.58 | 1.55 | 1.56 | 0 | 2.04 |
| 14 | 1.3 | 0 | 1.57 | 0 | 1.4 | 0 | 0 | 1.75 | 0 | 0 | 0 | 0 | 0 | 0 | 0 | 0 | 0 |
| 15 | 0 | 0 | 0 | 0 | 0 | 0 | 0 | 0 | 0 | 0 | 0 | 0 | 0 | 0 | 0 | 0 | 0 |
| 16 | 0 | 0 | 0 | 0 | 0 | 0 | 0.12 | 0 | 0 | 0 | 0 | 0.24 | 1.05 | 0.65 | 0.75 | 0 | 1.35 |
| 17 | 0 | 0 | 0 | 0 | 0 | 0 | 0 | 0 | 0 | 0 | 0 | 0 | 0 | 0 | 0 | 0 | 0.02 |
| 18 | 0 | 0.53 | 0 | 0 | 0 | 0 | 1.8 | 0 | 0 | 0 | 0 | 1.6 | 1.66 | 2.02 | 1.61 | 0.3 | 2.09 |
| 19 | 0.53 | 0 | 0 | 0 | 0.29 | 0 | 0 | 1.25 | 0 | 0 | 0 | 0 | 0 | 0 | 0 | 0 | 0 |
| 20 | 0 | 0 | 0 | 0 | 0 | 0 | 1.34 | 0 | 0 | 0 | 0 | 1.11 | 1.48 | 1.52 | 1.81 | 0.13 | 2.03 |
| 21 | 0 | 0 | 0 | 0 | 0 | 0 | 0 | 0 | 0 | 0 | 0 | 0 | 0 | 0 | 0 | 0 | 0 |
| 22 | 0 | 0.29 | 0 | 0 | 0 | 0 | 0 | 0 | 0 | 0 | 0 | 0.84 | 0.49 | 1.13 | 1.43 | 0 | 2.06 |
| 23 | 0 | 0 | 0 | 0 | 0 | 0 | 0 | 0 | 0 | 0 | 0 | 0 | 0 | 0 | 0 | 0 | 0 |
| 24 | 1.8 | 0 | 1.34 | 0 | 0 | 0 | 0 | 0 | 0 | 0 | 0 | 0 | 0 | 0 | 0 | 0 | 0 |
| 25 | 0 | 1.25 | 0 | 0 | 0 | 0 | 0 | 0 | 0 | 0 | 0 | 0.14 | 1.44 | 1.48 | 1.6 | 0.4 | 2.1 |
| 26 | 0 | 0 | 0 | 0 | 0 | 0 | 0 | 0 | 0 | 0 | 0 | 0 | 0 | 0 | 0 | 0 | 0 |
| 27 | 0 | 0 | 0 | 0 | 0 | 0 | 0 | 0 | 0 | 0 | 0 | 0 | 0 | 0 | 0 | 0 | 0.03 |
| 28 | 0 | 0 | 0 | 0 | 0 | 0 | 0 | 0 | 0 | 0 | 0 | 0 | 0 | 0 | 0 | 0 | 0 |
| 29 | 1.6 | 0 | 1.11 | 0 | 0.84 | 0 | 0 | 0.14 | 0 | 0 | 0 | 0 | 0 | 0 | 0 | 0 | 0 |
| 30 | 1.66 | 0 | 1.48 | 0 | 0.49 | 0 | 0 | 1.44 | 0 | 0 | 0 | 0 | 0 | 0 | 0 | 0 | 0 |
| 31 | 2.02 | 0 | 1.52 | 0 | 1.13 | 0 | 0 | 1.48 | 0 | 0 | 0 | 0 | 0 | 0 | 0 | 0 | 0 |
| 32 | 1.61 | 0 | 1.81 | 0 | 1.43 | 0 | 0 | 1.6 | 0 | 0 | 0 | 0 | 0 | 0 | 0 | 0 | 0 |
| 33 | 0.3 | 0 | 0.13 | 0 | 0 | 0 | 0 | 0.4 | 0 | 0 | 0 | 0 | 0 | 0 | 0 | 0 | 0 |
| 34 | 2.09 | 0 | 2.03 | 0 | 2.06 | 0 | 0 | 2.1 | 0 | 0.03 | 0 | 0 | 0 | 0 | 0 | 0 | 0 |
| 35 | 0.56 | 0 | 1.09 | 0 | 0 | 0 | 0 | 0.06 | 0 | 0 | 0 | 0 | 0 | 0 | 0 | 0 | 0 |
| 36 | 0 | 0 | 0 | 0 | 0 | 0 | 0 | 0 | 0 | 0 | 0 | 0 | 0 | 0 | 0 | 0 | 0 |
| 37 | 0 | 0 | 0 | 0 | 0 | 0 | 0 | 0 | 0 | 0 | 0 | 0 | 0 | 0 | 0 | 0 | 0 |
| 38 | 0 | 1.18 | 0 | 0 | 0 | 0 | 1.9 | 0 | 0 | 0 | 0 | 0.81 | 1.12 | 1.13 | 1.06 | 0 | 0.48 |
| 39 | 0 | 0 | 0 | 0 | 0 | 0 | 0 | 0 | 0 | 0 | 0 | 0 | 0 | 0 | 0 | 0 | 0 |
| 40 | 0 | 0 | 0 | 0 | 0 | 0 | 0 | 0 | 0 | 0 | 0 | 0 | 0 | 0 | 0 | 0 | 0 |
| 41 | 0 | 0 | 0 | 0 | 0 | 0 | 0 | 0 | 0 | 0 | 0 | 0 | 0 | 0 | 0 | 0 | 0 |
| 42 | 2.11 | 0 | 1.93 | 0 | 1.98 | 0.05 | 0 | 2.12 | 0 | 0.01 | 0 | 0 | 0 | 0 | 0 | 0 | 0 |
| 43 | 1.86 | 0 | 1.85 | 0 | 0.96 | 0 | 0 | 1.26 | 0 | 0.01 | 0 | 0 | 0 | 0 | 0 | 0 | 0 |
| 44 | 0 | 0 | 0 | 0 | 0 | 0 | 0 | 0 | 0 | 0 | 0 | 0 | 0 | 0 | 0 | 0 | 0 |
| 45 | 2.05 | 0 | 2.05 | 0 | 1.68 | 0 | 0 | 2.05 | 0 | 0.56 | 0 | 0 | 0 | 0 | 0 | 0 | 0 |
| 46 | 1.79 | 0 | 1.72 | 0 | 0.87 | 0 | 0 | 1.45 | 0 | 0.07 | 0 | 0 | 0 | 0 | 0 | 0 | 0 |
| 47 | 0 | 0 | 0 | 0 | 0 | 0 | 0.96 | 0 | 0 | 0 | 0 | 0.09 | 1.28 | 0.95 | 1.61 | 0 | 1.43 |
| 48 | 0 | 0 | 0 | 0 | 0 | 0 | 0 | 0 | 0 | 0 | 0 | 0 | 0 | 0 | 0 | 0 | 0 |
| 49 | 0.61 | 0 | 0.02 | 0 | 0 | 0 | 1.66 | 0 | 0 | 0 | 0 | 0.01 | 0.76 | 0.89 | 0 | 0.04 | 1.23 |
| 50 | 2.17 | 0 | 2.08 | 0 | 2.02 | 0 | 0 | 2.09 | 0 | 0.15 | 0 | 0 | 0 | 0 | 0 | 0 | 0 |

Continued table S1

| | 35 | 36 | 37 | 38 | 39 | 40 | 41 | 42 | 43 | 44 | 45 | 46 | 47 | 48 | 49 | 50 |
|---|---|---|---|---|---|---|---|---|---|---|---|---|---|---|---|---|
| 1 | 0 | 0 | 0 | 0 | 0 | 0 | 0 | 0.72 | 0.08 | 0 | 1.01 | 0 | 0 | 0 | 0 | 0.47 |
| 2 | 1.03 | 0.5 | 0 | 1.34 | 0 | 0 | 0 | 2.05 | 1.34 | 0 | 1.73 | 1.08 | 1.49 | 0 | 1.12 | 2.01 |
| 3 | 0 | 0.94 | 0 | 2.05 | 0 | 0 | 0 | 0 | 0 | 0 | 0 | 0 | 0.33 | 0 | 0.22 | 0 |
| 4 | 0 | 0 | 0 | 0 | 0 | 0 | 0 | 0 | 0 | 0 | 0 | 0 | 0 | 0 | 0 | 0 |
| 5 | 1.45 | 0 | 0 | 0 | 0 | 0 | 0 | 2.08 | 1.91 | 0 | 1.85 | 1.91 | 0 | 0 | 0 | 2.14 |
| 6 | 0 | 0 | 0 | 0 | 0 | 0 | 0 | 1.05 | 0 | 0 | 1.02 | 0 | 0 | 0 | 0 | 0.94 |
| 7 | 0.96 | 0.62 | 0 | 1.3 | 0 | 0 | 0 | 1.42 | 0 | 0 | 1.28 | 0 | 0.42 | 0 | 0 | 1.52 |
| 8 | 0 | 0 | 0 | 0 | 0 | 0 | 0 | 1.09 | 0.34 | 0 | 1.06 | 0.41 | 0 | 0 | 0 | 0.88 |
| 9 | 0 | 0.27 | 0 | 1.01 | 0 | 0 | 0 | 0.85 | 0.96 | 0 | 1.57 | 0.64 | 0.14 | 0 | 0 | 1.25 |
| 10 | 0 | 1.39 | 0 | 2.11 | 0 | 0 | 0 | 0 | 0 | 0 | 0 | 0 | 1.22 | 0 | 1.4 | 0 |
| 11 | 1.66 | 0.19 | 0 | 1.18 | 0 | 0 | 0 | 2.03 | 1.65 | 0 | 1.72 | 1.19 | 0 | 0 | 0.98 | 2.05 |
| 12 | 0 | 0 | 0 | 0 | 0 | 0 | 0 | 0 | 0 | 0 | 0 | 0 | 0 | 0 | 0 | 0 |
| 13 | 0.42 | 0 | 0 | 0 | 0 | 0 | 0 | 2.07 | 1.18 | 0 | 1.9 | 1.8 | 0 | 0 | 0 | 2.15 |
| 14 | 0 | 0.14 | 0 | 2.03 | 0 | 0 | 0 | 0 | 0 | 0 | 0 | 0 | 1.58 | 0 | 0.82 | 0 |
| 15 | 0 | 0 | 0 | 0 | 0 | 0 | 0 | 0 | 0 | 0 | 0 | 0 | 0 | 0 | 0 | 0 |
| 16 | 0 | 0.05 | 0 | 0 | 0 | 0 | 0 | 1.7 | 0.72 | 0 | 1 | 0.05 | 0 | 0 | 0.43 | 0.12 |
| 17 | 0 | 0 | 0 | 0 | 0 | 0 | 0 | 0 | 0 | 0 | 0 | 0 | 0 | 0 | 0 | 0 |
| 18 | 0.56 | 0 | 0 | 0 | 0 | 0 | 0 | 2.11 | 1.86 | 0 | 2.05 | 1.79 | 0 | 0 | 0.61 | 2.17 |
| 19 | 0 | 0 | 0 | 1.18 | 0 | 0 | 0 | 0 | 0 | 0 | 0 | 0 | 0 | 0 | 0 | 0 |
| 20 | 1.09 | 0 | 0 | 0 | 0 | 0 | 0 | 1.93 | 1.85 | 0 | 2.05 | 1.72 | 0 | 0 | 0.02 | 2.08 |
| 21 | 0 | 0 | 0 | 0 | 0 | 0 | 0 | 0 | 0 | 0 | 0 | 0 | 0 | 0 | 0 | 0 |
| 22 | 0 | 0 | 0 | 0 | 0 | 0 | 0 | 1.98 | 0.96 | 0 | 1.68 | 0.87 | 0 | 0 | 0 | 2.02 |
| 23 | 0 | 0 | 0 | 0 | 0 | 0 | 0 | 0.05 | 0 | 0 | 0 | 0 | 0 | 0 | 0 | 0 |
| 24 | 0 | 0 | 0 | 1.9 | 0 | 0 | 0 | 0 | 0 | 0 | 0 | 0 | 0.96 | 0 | 1.66 | 0 |
| 25 | 0.06 | 0 | 0 | 0 | 0 | 0 | 0 | 2.12 | 1.26 | 0 | 2.05 | 1.45 | 0 | 0 | 0 | 2.09 |
| 26 | 0 | 0 | 0 | 0 | 0 | 0 | 0 | 0 | 0 | 0 | 0 | 0 | 0 | 0 | 0 | 0 |
| 27 | 0 | 0 | 0 | 0 | 0 | 0 | 0 | 0.01 | 0.01 | 0 | 0.56 | 0.07 | 0 | 0 | 0 | 0.15 |
| 28 | 0 | 0 | 0 | 0 | 0 | 0 | 0 | 0 | 0 | 0 | 0 | 0 | 0 | 0 | 0 | 0 |
| 29 | 0 | 0 | 0 | 0.81 | 0 | 0 | 0 | 0 | 0 | 0 | 0 | 0 | 0.09 | 0 | 0.01 | 0 |
| 30 | 0 | 0 | 0 | 1.12 | 0 | 0 | 0 | 0 | 0 | 0 | 0 | 0 | 1.28 | 0 | 0.76 | 0 |
| 31 | 0 | 0 | 0 | 1.13 | 0 | 0 | 0 | 0 | 0 | 0 | 0 | 0 | 0.95 | 0 | 0.89 | 0 |
| 32 | 0 | 0 | 0 | 1.06 | 0 | 0 | 0 | 0 | 0 | 0 | 0 | 0 | 1.61 | 0 | 0 | 0 |
| 33 | 0 | 0 | 0 | 0 | 0 | 0 | 0 | 0 | 0 | 0 | 0 | 0 | 0 | 0 | 0.04 | 0 |
| 34 | 0 | 0 | 0 | 0.48 | 0 | 0 | 0 | 0 | 0 | 0 | 0 | 0 | 1.43 | 0 | 1.23 | 0 |
| 35 | 0 | 0 | 0 | 0 | 0 | 0 | 0 | 0 | 0 | 0 | 0 | 0 | 0.17 | 0 | 0 | 0 |
| 36 | 0 | 0 | 0 | 0 | 0 | 0 | 0 | 0 | 0 | 0 | 0.17 | 0 | 0 | 0 | 0 | 0.29 |
| 37 | 0 | 0 | 0 | 0 | 0 | 0 | 0 | 0 | 0 | 0 | 0 | 0 | 0 | 0 | 0 | 0 |
| 38 | 0 | 0 | 0 | 0 | 0 | 0 | 0 | 0.19 | 0.31 | 0 | 1.39 | 0.85 | 0 | 0 | 0 | 2.08 |
| 39 | 0 | 0 | 0 | 0 | 0 | 0 | 0 | 0 | 0 | 0 | 0 | 0 | 0 | 0 | 0 | 0 |
| 40 | 0 | 0 | 0 | 0 | 0 | 0 | 0 | 0 | 0 | 0 | 0 | 0 | 0 | 0 | 0 | 0 |
| 41 | 0 | 0 | 0 | 0 | 0 | 0 | 0 | 0 | 0 | 0 | 0 | 0 | 0 | 0 | 0 | 0 |
| 42 | 0 | 0 | 0 | 0.19 | 0 | 0 | 0 | 0 | 0 | 0 | 0 | 0 | 0.85 | 0 | 0.28 | 0 |
| 43 | 0 | 0 | 0 | 0.31 | 0 | 0 | 0 | 0 | 0 | 0 | 0 | 0 | 0 | 0 | 0 | 0 |
| 44 | 0 | 0 | 0 | 0 | 0 | 0 | 0 | 0 | 0 | 0 | 0 | 0 | 0 | 0 | 0 | 0 |
| 45 | 0 | 0.17 | 0 | 1.39 | 0 | 0 | 0 | 0 | 0 | 0 | 0 | 0 | 0 | 0 | 0 | 0 |
| 46 | 0 | 0 | 0 | 0.85 | 0 | 0 | 0 | 0 | 0 | 0 | 0 | 0 | 0 | 0 | 0 | 0 |
| 47 | 0.17 | 0 | 0 | 0 | 0 | 0 | 0 | 0.85 | 0 | 0 | 0 | 0 | 0 | 0 | 0 | 0 |
| 48 | 0 | 0 | 0 | 0 | 0 | 0 | 0 | 0 | 0 | 0 | 0 | 0 | 0 | 0 | 0 | 0 |
| 49 | 0 | 0 | 0 | 0 | 0 | 0 | 0 | 0.28 | 0 | 0 | 0 | 0 | 0 | 0 | 0 | 0 |
| 50 | 0 | 0.29 | 0 | 2.08 | 0 | 0 | 0 | 0 | 0 | 0 | 0 | 0 | 0 | 0 | 0 | 0 |

**Table S2:** Optimized interaction strength matrix for K562 (ON state) cell line at the normalizing factor $N_f = 0$. The first row and the first column indicates the bead number ($\mu$ or $\nu$) and all the remaining elements represent the attractive strength between the corresponding bead pairs ($\epsilon_{\mu\nu}$).

| | 1 | 2 | 3 | 4 | 5 | 6 | 7 | 8 | 9 | 10 | 11 | 12 | 13 | 14 | 15 | 16 | 17 |
|---|---|---|---|---|---|---|---|---|---|---|---|---|---|---|---|---|---|
| 1 | 0 | 0 | 0 | 0 | 0 | 0 | 0 | 0 | 0 | 0.06 | 0 | 0 | 0 | 0.78 | 0 | 0 | 0 |
| 2 | 0 | 0 | 0 | 0 | 0 | 0 | 0 | 0 | 0.11 | 0.32 | 0 | 0 | 0 | 0 | 0 | 0 | 0.04 |
| 3 | 0 | 0 | 0 | 0 | 0 | 0 | 0 | 0 | 0 | 0 | 0 | 0 | 0.01 | 0 | 0 | 0.03 | 0 |
| 4 | 0 | 0 | 0 | 0 | 0 | 0 | 0 | 0 | 0 | 0 | 0 | 0 | 0 | 0 | 0 | 0 | 0 |
| 5 | 0 | 0 | 0 | 0 | 0 | 0 | 0 | 0 | 0 | 1.46 | 0 | 0 | 0 | 0.61 | 0 | 0 | 0 |
| 6 | 0 | 0 | 0 | 0 | 0 | 0 | 0 | 0 | 0 | 0 | 0 | 0 | 0 | 0 | 0 | 0 | 0 |
| 7 | 0 | 0 | 0 | 0 | 0 | 0 | 0 | 0 | 0 | 0 | 0 | 0 | 0 | 0 | 0 | 0 | 0 |
| 8 | 0 | 0 | 0 | 0 | 0 | 0 | 0 | 0 | 0 | 0 | 0 | 0 | 0 | 0 | 0 | 0 | 0 |
| 9 | 0 | 0.11 | 0 | 0 | 0 | 0 | 0 | 0 | 0 | 1.49 | 0 | 0 | 0 | 0 | 0 | 0 | 0 |
| 10 | 0.06 | 0.32 | 0 | 0 | 1.46 | 0 | 0 | 0 | 1.49 | 0 | 0 | 0 | 0.74 | 0 | 0 | 1.57 | 0 |
| 11 | 0 | 0 | 0 | 0 | 0 | 0 | 0 | 0 | 0 | 0 | 0 | 0 | 0 | 0 | 0 | 0 | 0 |
| 12 | 0 | 0 | 0 | 0 | 0 | 0 | 0 | 0 | 0 | 0 | 0 | 0 | 0 | 0 | 0 | 0 | 0 |
| 13 | 0 | 0 | 0.01 | 0 | 0 | 0 | 0 | 0 | 0 | 0.74 | 0 | 0 | 0 | 0 | 0 | 0 | 0 |
| 14 | 0.78 | 0 | 0 | 0 | 0.61 | 0 | 0 | 0 | 0 | 0 | 0 | 0 | 0 | 0 | 0 | 0 | 0 |
| 15 | 0 | 0 | 0 | 0 | 0 | 0 | 0 | 0 | 0 | 0 | 0 | 0 | 0 | 0 | 0 | 0 | 0 |
| 16 | 0 | 0 | 0.03 | 0 | 0 | 0 | 0 | 0 | 0 | 1.57 | 0 | 0 | 0 | 0 | 0 | 0 | 0 |
| 17 | 0 | 0.04 | 0 | 0 | 0 | 0 | 0 | 0 | 0 | 0 | 0 | 0 | 0 | 0 | 0 | 0 | 0 |
| 18 | 0 | 1.38 | 1.85 | 0 | 0 | 0.62 | 0.23 | 0 | 0.13 | 3.06 | 0.06 | 0 | 0 | 0 | 0 | 0 | 0 |
| 19 | 0 | 0 | 0 | 0 | 1.07 | 0 | 1.4 | 0 | 0 | 0 | 0 | 0 | 0 | 0 | 0 | 0 | 0 |
| 20 | 0 | 0.08 | 1.48 | 0 | 0 | 0.14 | 0.44 | 0 | 0.07 | 2.05 | 0.13 | 0 | 0 | 0 | 0 | 0 | 0 |
| 21 | 0 | 0 | 0 | 0 | 0 | 0 | 0 | 0 | 0 | 0 | 0 | 0 | 0 | 0 | 0 | 0 | 0 |
| 22 | 0 | 0.93 | 0.14 | 0 | 0 | 0 | 0 | 0 | 0 | 1.9 | 0 | 0 | 0 | 0 | 0 | 0 | 0 |
| 23 | 0 | 0 | 0.04 | 0 | 0 | 0 | 0 | 0 | 0 | 0 | 0.03 | 0 | 0 | 0 | 0 | 0 | 0 |
| 24 | 0 | 0 | 0 | 0 | 0.04 | 0 | 0 | 0.28 | 0 | 0 | 0 | 0 | 0 | 0 | 0 | 0 | 0 |
| 25 | 0 | 0.16 | 1.97 | 0 | 0 | 0.01 | 0 | 0 | 0.24 | 2.06 | 0.12 | 0 | 0 | 0.71 | 0 | 0 | 0 |
| 26 | 0 | 0 | 0 | 0 | 0 | 0 | 0 | 0 | 0 | 0 | 0 | 0 | 0 | 0 | 0 | 0 | 0 |
| 27 | 0 | 0 | 0 | 0 | 0 | 0 | 0 | 0 | 0 | 0.34 | 0 | 0 | 0 | 0 | 0 | 0 | 0 |
| 28 | 0 | 0 | 0 | 0 | 0 | 0 | 0 | 0 | 0 | 0 | 0 | 0 | 0 | 0 | 0 | 0 | 0 |
| 29 | 0 | 0 | 0 | 0 | 0 | 0 | 0.11 | 0 | 0 | 0 | 0 | 0 | 0 | 0 | 0 | 0 | 0 |
| 30 | 0.44 | 0.54 | 0 | 0 | 2.06 | 0 | 0.78 | 0.08 | 0.94 | 0 | 1.11 | 0 | 0 | 0 | 0 | 0 | 0 |
| 31 | 0.4 | 0 | 0 | 0 | 1.05 | 0.05 | 0.08 | 0 | 0.55 | 0 | 1.8 | 0 | 1.79 | 0 | 0 | 0.02 | 0 |
| 32 | 0 | 0 | 0 | 0 | 1.7 | 0 | 0.59 | 0 | 0 | 0 | 0.01 | 0 | 0 | 0 | 0 | 0 | 0 |
| 33 | 0 | 0 | 0 | 0 | 0.08 | 0 | 0 | 0 | 0 | 0 | 0 | 0 | 0 | 0 | 0 | 0 | 0 |
| 34 | 2.54 | 1.91 | 0 | 0 | 1.93 | 0.97 | 1.7 | 1.61 | 1.15 | 0 | 1.92 | 0 | 0.65 | 0 | 0 | 0 | 0 |
| 35 | 0 | 0 | 0 | 0 | 0 | 0 | 0.32 | 0 | 0 | 0 | 0 | 0 | 0 | 0 | 0 | 0 | 0 |
| 36 | 0 | 0 | 0 | 0 | 0.36 | 0 | 0 | 0 | 0 | 0.3 | 0.01 | 0 | 0 | 0 | 0 | 0 | 0 |
| 37 | 0 | 0 | 0 | 0 | 0 | 0 | 0 | 0 | 0 | 0 | 0 | 0 | 0 | 0 | 0 | 0 | 0 |
| 38 | 0 | 0 | 0.78 | 0 | 0 | 0 | 1.21 | 0 | 0 | 1.96 | 0.7 | 0 | 0 | 0 | 0 | 0 | 0 |
| 39 | 0 | 0 | 0 | 0 | 0 | 0 | 0 | 0 | 0 | 0 | 0 | 0 | 0 | 0 | 0 | 0 | 0 |
| 40 | 0 | 0 | 0 | 0 | 0 | 0 | 0 | 0 | 0 | 0 | 0 | 0 | 0 | 0 | 0 | 0 | 0 |
| 41 | 0 | 0 | 0 | 0 | 0 | 0 | 0 | 0 | 0 | 0 | 0 | 0 | 0 | 0 | 0 | 0 | 0 |
| 42 | 0 | 0 | 0 | 0 | 0 | 0 | 0 | 0 | 0 | 0 | 0.93 | 0 | 1.18 | 0 | 0 | 1.05 | 0 |
| 43 | 0 | 0 | 0 | 0 | 0 | 0 | 1.45 | 0 | 0 | 0 | 0 | 0 | 0 | 0 | 0 | 0 | 0 |
| 44 | 0 | 0 | 0 | 0 | 0 | 0 | 0 | 0 | 0 | 0 | 0 | 0 | 0 | 0 | 0 | 0 | 0 |
| 45 | 0 | 0 | 0 | 0 | 0 | 0 | 0 | 1.31 | 0 | 0 | 0 | 0 | 0 | 0 | 0 | 0 | 0 |
| 46 | 0 | 0 | 0 | 0 | 1.66 | 0 | 0 | 0.85 | 0 | 0 | 0 | 0 | 2.11 | 0 | 0 | 0 | 0 |
| 47 | 0 | 0 | 0 | 0 | 0 | 0 | 0 | 0 | 0.44 | 1.33 | 0 | 0 | 0 | 0 | 0 | 0 | 0 |
| 48 | 0 | 0 | 0 | 0 | 0 | 0 | 0 | 0 | 0 | 0 | 0 | 0 | 0 | 0 | 0 | 0 | 0 |
| 49 | 0.97 | 1.23 | 0 | 0 | 0 | 0 | 0 | 0 | 0 | 1.15 | 1.83 | 0 | 0 | 0 | 0 | 0 | 0 |
| 50 | 0 | 0 | 0 | 0 | 1.76 | 0 | 1.81 | 1.57 | 1.23 | 0 | 0 | 0 | 0 | 0 | 0 | 0 | 0 |

Continued table S2

| | 18 | 19 | 20 | 21 | 22 | 23 | 24 | 25 | 26 | 27 | 28 | 29 | 30 | 31 | 32 | 33 | 34 |
|---|---|---|---|---|---|---|---|---|---|---|---|---|---|---|---|---|---|
| 1 | 0 | 0 | 0 | 0 | 0 | 0 | 0 | 0 | 0 | 0 | 0 | 0 | 0.44 | 0.4 | 0 | 0 | 2.54 |
| 2 | 1.38 | 0 | 0.08 | 0 | 0.93 | 0 | 0 | 0.16 | 0 | 0 | 0 | 0 | 0.54 | 0 | 0 | 0 | 1.91 |
| 3 | 1.85 | 0 | 1.48 | 0 | 0.14 | 0.04 | 0 | 1.97 | 0 | 0 | 0 | 0 | 0 | 0 | 0 | 0 | 0 |
| 4 | 0 | 0 | 0 | 0 | 0 | 0 | 0 | 0 | 0 | 0 | 0 | 0 | 0 | 0 | 0 | 0 | 0 |
| 5 | 0 | 1.07 | 0 | 0 | 0 | 0 | 0.04 | 0 | 0 | 0 | 0 | 0 | 2.06 | 1.05 | 1.7 | 0.08 | 1.93 |
| 6 | 0.62 | 0 | 0.14 | 0 | 0 | 0 | 0 | 0.01 | 0 | 0 | 0 | 0 | 0 | 0.05 | 0 | 0 | 0.97 |
| 7 | 0.23 | 1.4 | 0.44 | 0 | 0 | 0 | 0 | 0 | 0 | 0 | 0 | 0.11 | 0.78 | 0.08 | 0.59 | 0 | 1.7 |
| 8 | 0 | 0 | 0 | 0 | 0 | 0 | 0.28 | 0 | 0 | 0 | 0 | 0 | 0.08 | 0 | 0 | 0 | 1.61 |
| 9 | 0.13 | 0 | 0.07 | 0 | 0 | 0 | 0 | 0.24 | 0 | 0 | 0 | 0 | 0.94 | 0.55 | 0 | 0 | 1.15 |
| 10 | 3.06 | 0 | 2.05 | 0 | 1.9 | 0 | 0 | 2.06 | 0 | 0.34 | 0 | 0 | 0 | 0 | 0 | 0 | 0 |
| 11 | 0.06 | 0 | 0.13 | 0 | 0 | 0.03 | 0 | 0.12 | 0 | 0 | 0 | 0 | 1.11 | 1.8 | 0.01 | 0 | 1.92 |
| 12 | 0 | 0 | 0 | 0 | 0 | 0 | 0 | 0 | 0 | 0 | 0 | 0 | 0 | 0 | 0 | 0 | 0 |
| 13 | 0 | 0 | 0 | 0 | 0 | 0 | 0 | 0 | 0 | 0 | 0 | 0 | 0 | 1.79 | 0 | 0 | 0.65 |
| 14 | 0 | 0 | 0 | 0 | 0 | 0 | 0 | 0.71 | 0 | 0 | 0 | 0 | 0 | 0 | 0 | 0 | 0 |
| 15 | 0 | 0 | 0 | 0 | 0 | 0 | 0 | 0 | 0 | 0 | 0 | 0 | 0 | 0 | 0 | 0 | 0 |
| 16 | 0 | 0 | 0 | 0 | 0 | 0 | 0 | 0 | 0 | 0 | 0 | 0 | 0 | 0.02 | 0 | 0 | 0 |
| 17 | 0 | 0 | 0 | 0 | 0 | 0 | 0 | 0 | 0 | 0 | 0 | 0 | 0 | 0 | 0 | 0 | 0 |
| 18 | 0 | 1.4 | 0 | 0 | 0 | 0 | 0 | 0 | 0 | 0 | 0 | 0.15 | 1.69 | 1.54 | 0.56 | 0 | 2.39 |
| 19 | 1.4 | 0 | 0 | 0 | 0 | 0 | 0 | 0.46 | 0 | 0 | 0 | 0 | 0 | 0 | 0 | 0 | 0 |
| 20 | 0 | 0 | 0 | 0 | 0 | 0 | 0 | 0 | 0 | 0 | 0 | 0 | 1.39 | 1.93 | 0.83 | 0 | 2.2 |
| 21 | 0 | 0 | 0 | 0 | 0 | 0 | 0 | 0 | 0 | 0 | 0 | 0 | 0 | 0 | 0 | 0 | 0 |
| 22 | 0 | 0 | 0 | 0 | 0 | 0 | 0 | 0 | 0 | 0 | 0 | 0 | 0.69 | 1.02 | 0.64 | 0 | 1.29 |
| 23 | 0 | 0 | 0 | 0 | 0 | 0 | 0 | 0 | 0 | 0 | 0 | 0 | 0 | 0 | 0 | 0 | 0 |
| 24 | 0 | 0 | 0 | 0 | 0 | 0 | 0 | 1.46 | 0 | 0 | 0 | 0 | 0 | 0 | 0 | 0 | 0 |
| 25 | 0 | 0.46 | 0 | 0 | 0 | 0 | 1.46 | 0 | 0 | 0 | 0 | 0 | 1.02 | 0.18 | 1.12 | 0 | 1.66 |
| 26 | 0 | 0 | 0 | 0 | 0 | 0 | 0 | 0 | 0 | 0 | 0 | 0 | 0 | 0 | 0 | 0 | 0 |
| 27 | 0 | 0 | 0 | 0 | 0 | 0 | 0 | 0 | 0 | 0 | 0 | 0 | 0 | 0 | 0 | 0 | 0 |
| 28 | 0 | 0 | 0 | 0 | 0 | 0 | 0 | 0 | 0 | 0 | 0 | 0 | 0 | 0 | 0 | 0 | 0 |
| 29 | 0.15 | 0 | 0 | 0 | 0 | 0 | 0 | 0 | 0 | 0 | 0 | 0 | 0 | 0 | 0 | 0 | 0 |
| 30 | 1.69 | 0 | 1.39 | 0 | 0.69 | 0 | 0 | 1.02 | 0 | 0 | 0 | 0 | 0 | 0 | 0 | 0 | 0 |
| 31 | 1.54 | 0 | 1.93 | 0 | 1.02 | 0 | 0 | 0.18 | 0 | 0 | 0 | 0 | 0 | 0 | 0 | 0 | 0 |
| 32 | 0.56 | 0 | 0.83 | 0 | 0.64 | 0 | 0 | 1.12 | 0 | 0 | 0 | 0 | 0 | 0 | 0 | 0 | 0 |
| 33 | 0 | 0 | 0 | 0 | 0 | 0 | 0 | 0 | 0 | 0 | 0 | 0 | 0 | 0 | 0 | 0 | 0 |
| 34 | 2.39 | 0 | 2.2 | 0 | 1.29 | 0 | 0 | 1.66 | 0 | 0 | 0 | 0 | 0 | 0 | 0 | 0 | 0 |
| 35 | 0 | 0 | 0 | 0 | 0 | 0 | 0 | 0 | 0 | 0 | 0 | 0 | 0 | 0 | 0 | 0 | 0 |
| 36 | 0 | 0 | 0 | 0 | 0 | 0 | 0 | 0 | 0 | 0 | 0 | 0 | 0 | 0 | 0 | 0 | 0 |
| 37 | 0 | 0 | 0 | 0 | 0 | 0 | 0 | 0 | 0 | 0 | 0 | 0 | 0 | 0 | 0 | 0 | 0 |
| 38 | 0 | 0.07 | 0 | 0 | 0 | 0 | 0 | 0 | 0 | 0 | 0 | 0 | 0 | 0 | 0 | 0 | 0 |
| 39 | 0 | 0 | 0 | 0 | 0 | 0 | 0 | 0 | 0 | 0 | 0 | 0 | 0 | 0 | 0 | 0 | 0 |
| 40 | 0 | 0 | 0 | 0 | 0 | 0 | 0 | 0 | 0 | 0 | 0 | 0 | 0 | 0 | 0 | 0 | 0 |
| 41 | 0 | 0 | 0 | 0 | 0 | 0 | 0 | 0 | 0 | 0 | 0 | 0 | 0 | 0 | 0 | 0 | 0 |
| 42 | 0.5 | 0 | 0.85 | 0 | 0.86 | 0 | 0 | 1.17 | 0 | 0 | 0 | 0 | 0 | 0 | 0 | 0 | 0 |
| 43 | 1.94 | 0 | 1.56 | 0 | 0.03 | 0 | 0 | 0.9 | 0 | 0 | 0 | 0 | 0 | 0 | 0 | 0 | 0 |
| 44 | 0 | 0 | 0 | 0 | 0 | 0 | 0 | 0 | 0 | 0 | 0 | 0 | 0 | 0 | 0 | 0 | 0 |
| 45 | 0.48 | 0 | 1.09 | 0 | 0.62 | 0 | 0 | 1.21 | 0 | 0 | 0 | 0 | 0 | 0 | 0 | 0 | 0 |
| 46 | 1.26 | 0 | 0.79 | 0 | 1.17 | 0 | 0 | 1.21 | 0 | 0 | 0 | 0 | 0 | 0 | 0 | 0 | 0 |
| 47 | 0 | 0 | 0 | 0 | 0 | 0 | 0 | 0 | 0 | 0 | 0 | 0.19 | 0.02 | 1.18 | 0 | 0.01 | 0 |
| 48 | 0 | 0 | 0 | 0 | 0 | 0 | 0 | 0 | 0 | 0 | 0 | 0 | 0 | 0 | 0 | 0 | 0 |
| 49 | 0 | 0 | 0.03 | 0 | 0 | 0 | 0 | 1.02 | 0 | 0 | 0 | 0 | 0.01 | 0.92 | 0 | 0 | 0.08 |
| 50 | 2.25 | 0 | 1.63 | 0 | 1.66 | 0 | 0 | 0.45 | 0 | 0 | 0 | 0 | 0 | 0 | 0 | 0 | 0 |

Continued table S2

| | 35 | 36 | 37 | 38 | 39 | 40 | 41 | 42 | 43 | 44 | 45 | 46 | 47 | 48 | 49 | 50 |
|---|---|---|---|---|---|---|---|---|---|---|---|---|---|---|---|---|
| 1 | 0 | 0 | 0 | 0 | 0 | 0 | 0 | 0 | 0 | 0 | 0 | 0 | 0 | 0 | 0.97 | 0 |
| 2 | 0 | 0 | 0 | 0 | 0 | 0 | 0 | 0 | 0 | 0 | 0 | 0 | 0 | 0 | 1.23 | 0 |
| 3 | 0 | 0 | 0 | 0.78 | 0 | 0 | 0 | 0 | 0 | 0 | 0 | 0 | 0 | 0 | 0 | 0 |
| 4 | 0 | 0 | 0 | 0 | 0 | 0 | 0 | 0 | 0 | 0 | 0 | 0 | 0 | 0 | 0 | 0 |
| 5 | 0 | 0.36 | 0 | 0 | 0 | 0 | 0 | 0 | 0 | 0 | 0 | 1.66 | 0 | 0 | 0 | 1.76 |
| 6 | 0 | 0 | 0 | 0 | 0 | 0 | 0 | 0 | 0 | 0 | 0 | 0 | 0 | 0 | 0 | 0 |
| 7 | 0.32 | 0 | 0 | 1.21 | 0 | 0 | 0 | 0 | 1.45 | 0 | 0 | 0 | 0 | 0 | 0 | 1.81 |
| 8 | 0 | 0 | 0 | 0 | 0 | 0 | 0 | 0 | 0 | 0 | 1.31 | 0.85 | 0 | 0 | 0 | 1.57 |
| 9 | 0 | 0 | 0 | 0 | 0 | 0 | 0 | 0 | 0 | 0 | 0 | 0 | 0.44 | 0 | 0 | 1.23 |
| 10 | 0 | 0.3 | 0 | 1.96 | 0 | 0 | 0 | 0 | 0 | 0 | 0 | 0 | 1.33 | 0 | 1.15 | 0 |
| 11 | 0 | 0.01 | 0 | 0.7 | 0 | 0 | 0 | 0.93 | 0 | 0 | 0 | 0 | 0 | 0 | 1.83 | 0 |
| 12 | 0 | 0 | 0 | 0 | 0 | 0 | 0 | 0 | 0 | 0 | 0 | 0 | 0 | 0 | 0 | 0 |
| 13 | 0 | 0 | 0 | 0 | 0 | 0 | 0 | 1.18 | 0 | 0 | 0 | 2.11 | 0 | 0 | 0 | 0 |
| 14 | 0 | 0 | 0 | 0 | 0 | 0 | 0 | 0 | 0 | 0 | 0 | 0 | 0 | 0 | 0 | 0 |
| 15 | 0 | 0 | 0 | 0 | 0 | 0 | 0 | 0 | 0 | 0 | 0 | 0 | 0 | 0 | 0 | 0 |
| 16 | 0 | 0 | 0 | 0 | 0 | 0 | 0 | 1.05 | 0 | 0 | 0 | 0 | 0 | 0 | 0 | 0 |
| 17 | 0 | 0 | 0 | 0 | 0 | 0 | 0 | 0 | 0 | 0 | 0 | 0 | 0 | 0 | 0 | 0 |
| 18 | 0 | 0 | 0 | 0 | 0 | 0 | 0 | 0.5 | 1.94 | 0 | 0.48 | 1.26 | 0 | 0 | 0 | 2.25 |
| 19 | 0 | 0 | 0 | 0.07 | 0 | 0 | 0 | 0 | 0 | 0 | 0 | 0 | 0 | 0 | 0 | 0 |
| 20 | 0 | 0 | 0 | 0 | 0 | 0 | 0 | 0.85 | 1.56 | 0 | 1.09 | 0.79 | 0 | 0 | 0.03 | 1.63 |
| 21 | 0 | 0 | 0 | 0 | 0 | 0 | 0 | 0 | 0 | 0 | 0 | 0 | 0 | 0 | 0 | 0 |
| 22 | 0 | 0 | 0 | 0 | 0 | 0 | 0 | 0.86 | 0.03 | 0 | 0.62 | 1.17 | 0 | 0 | 0 | 1.66 |
| 23 | 0 | 0 | 0 | 0 | 0 | 0 | 0 | 0 | 0 | 0 | 0 | 0 | 0 | 0 | 0 | 0 |
| 24 | 0 | 0 | 0 | 0 | 0 | 0 | 0 | 0 | 0 | 0 | 0 | 0 | 0 | 0 | 0 | 0 |
| 25 | 0 | 0 | 0 | 0 | 0 | 0 | 0 | 1.17 | 0.9 | 0 | 1.21 | 1.21 | 0 | 0 | 1.02 | 0.45 |
| 26 | 0 | 0 | 0 | 0 | 0 | 0 | 0 | 0 | 0 | 0 | 0 | 0 | 0 | 0 | 0 | 0 |
| 27 | 0 | 0 | 0 | 0 | 0 | 0 | 0 | 0 | 0 | 0 | 0 | 0 | 0 | 0 | 0 | 0 |
| 28 | 0 | 0 | 0 | 0 | 0 | 0 | 0 | 0 | 0 | 0 | 0 | 0 | 0 | 0 | 0 | 0 |
| 29 | 0 | 0 | 0 | 0 | 0 | 0 | 0 | 0 | 0 | 0 | 0 | 0 | 0.19 | 0 | 0 | 0 |
| 30 | 0 | 0 | 0 | 0 | 0 | 0 | 0 | 0 | 0 | 0 | 0 | 0 | 0.02 | 0 | 0.01 | 0 |
| 31 | 0 | 0 | 0 | 0 | 0 | 0 | 0 | 0 | 0 | 0 | 0 | 0 | 1.18 | 0 | 0.92 | 0 |
| 32 | 0 | 0 | 0 | 0 | 0 | 0 | 0 | 0 | 0 | 0 | 0 | 0 | 0 | 0 | 0 | 0 |
| 33 | 0 | 0 | 0 | 0 | 0 | 0 | 0 | 0 | 0 | 0 | 0 | 0 | 0.01 | 0 | 0 | 0 |
| 34 | 0 | 0 | 0 | 0 | 0 | 0 | 0 | 0 | 0 | 0 | 0 | 0 | 0 | 0 | 0.08 | 0 |
| 35 | 0 | 0 | 0 | 0 | 0 | 0 | 0 | 0 | 0 | 0 | 0 | 0 | 0 | 0 | 0 | 0 |
| 36 | 0 | 0 | 0 | 0 | 0 | 0 | 0 | 0 | 0 | 0 | 0 | 0 | 0 | 0 | 0 | 0 |
| 37 | 0 | 0 | 0 | 0 | 0 | 0 | 0 | 0 | 0 | 0 | 0 | 0 | 0 | 0 | 0 | 0 |
| 38 | 0 | 0 | 0 | 0 | 0 | 0 | 0 | 0 | 0 | 0 | 0 | 0 | 0 | 0 | 0 | 0.76 |
| 39 | 0 | 0 | 0 | 0 | 0 | 0 | 0 | 0 | 0 | 0 | 0 | 0 | 0 | 0 | 0 | 0 |
| 40 | 0 | 0 | 0 | 0 | 0 | 0 | 0 | 0 | 0 | 0 | 0 | 0 | 0 | 0 | 0 | 0 |
| 41 | 0 | 0 | 0 | 0 | 0 | 0 | 0 | 0 | 0 | 0 | 0 | 0 | 0 | 0 | 0 | 0 |
| 42 | 0 | 0 | 0 | 0 | 0 | 0 | 0 | 0 | 0 | 0 | 0 | 0 | 0 | 0 | 0 | 0 |
| 43 | 0 | 0 | 0 | 0 | 0 | 0 | 0 | 0 | 0 | 0 | 0 | 0 | 0 | 0 | 0 | 0 |
| 44 | 0 | 0 | 0 | 0 | 0 | 0 | 0 | 0 | 0 | 0 | 0 | 0 | 0 | 0 | 0 | 0 |
| 45 | 0 | 0 | 0 | 0 | 0 | 0 | 0 | 0 | 0 | 0 | 0 | 0 | 0 | 0 | 0 | 0 |
| 46 | 0 | 0 | 0 | 0 | 0 | 0 | 0 | 0 | 0 | 0 | 0 | 0 | 0 | 0 | 0 | 0 |
| 47 | 0 | 0 | 0 | 0 | 0 | 0 | 0 | 0 | 0 | 0 | 0 | 0 | 0 | 0 | 0 | 0 |
| 48 | 0 | 0 | 0 | 0 | 0 | 0 | 0 | 0 | 0 | 0 | 0 | 0 | 0 | 0 | 0 | 0 |
| 49 | 0 | 0 | 0 | 0 | 0 | 0 | 0 | 0 | 0 | 0 | 0 | 0 | 0 | 0 | 0 | 0 |
| 50 | 0 | 0 | 0 | 0.76 | 0 | 0 | 0 | 0 | 0 | 0 | 0 | 0 | 0 | 0 | 0 | 0 |
